# Supplementary material for: Cheetah: Accelerating Database Queries with Switch Pruning
Source: arXiv:2004.05076 source file (2020-04-26)
Supplement: Supplementary file 1 [file appendix.tex]

\section{Appendix}

\subsection{distinct}
